# Supplementary material for: Observation of moir\'e trapped biexciton through sub-diffraction-limit probing using hetero-bilayer on nanopillar
Source: arXiv:2509.00879 source file (2025-08-31)
Supplement: Supplementary file 1 [file SI.pdf]

Supporting information for:

Observation of moiré trapped biexciton through  
sub-diffraction-limit probing using hetero-bilayer on nanopillar

Mayank Chhaperwal<sup>1,||</sup>, Suman Chatterjee<sup>1,2,||</sup>, Suchithra Puliassery<sup>1</sup>,  
Jyothsna Konkada Manattayil<sup>1</sup>, Rabindra Biswas<sup>1,3</sup>, Patrick Hays<sup>4</sup>, Seth Ariel Tongay<sup>4</sup>,  
Varun Raghunathan<sup>1</sup>, and Kausik Majumdar<sup>1\*</sup>

<sup>1</sup>Department of Electrical Communication Engineering,  
Indian Institute of Science, Bangalore 560012, India

<sup>2</sup>Currently at Quantum Matter Institute, University of British Columbia,  
Vancouver, British Columbia V6T 1Z4, Canada

<sup>3</sup>Currently at Department of Physics, Emory University, Atlanta, USA

<sup>4</sup>Materials Science and Engineering, School for Engineering of Matter,  
Transport and Energy, Arizona State University, Tempe, Arizona 85287, United States

<sup>||</sup>These authors contributed equally

\*Corresponding author, email: kausikm@iisc.ac.in

# Supporting Information 1 Polarization resolved SHG measurement

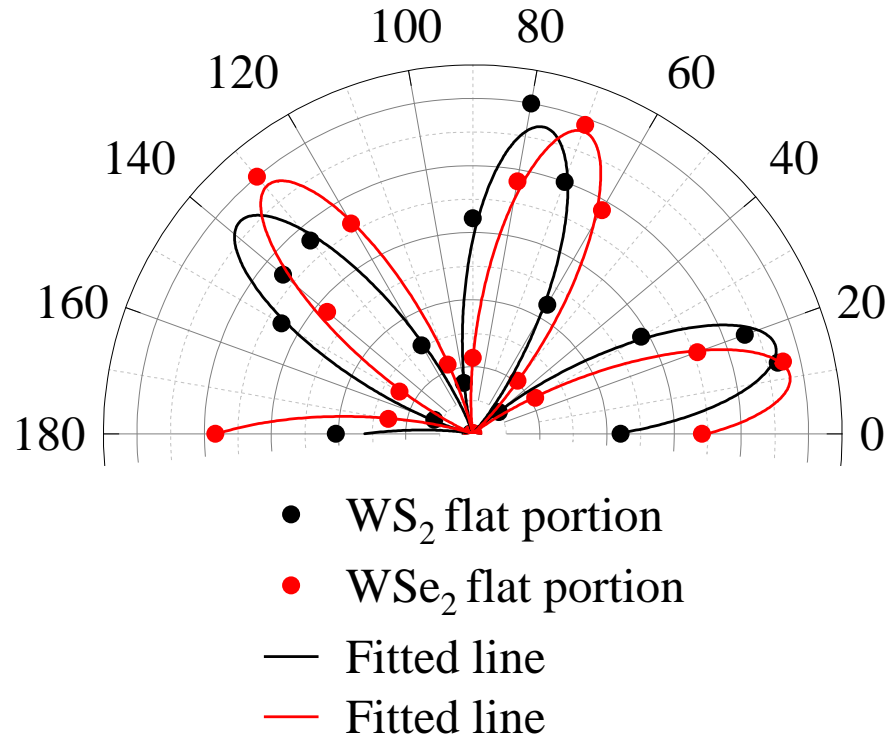

Supporting Figure 1: **Polarization resolved SHG measurement:** Red circles show the SHG intensity from the  $\text{WS}_2$  monolayer, and black squares show SHG intensity from  $\text{WSe}_2$  monolayer. Solid traces are fit to the data. Fit gives a relative twist angle of  $\sim 6^\circ$  between the two monolayers.

## Supporting Information 2 SHG enhancement on nanopillar compared to gold substrate

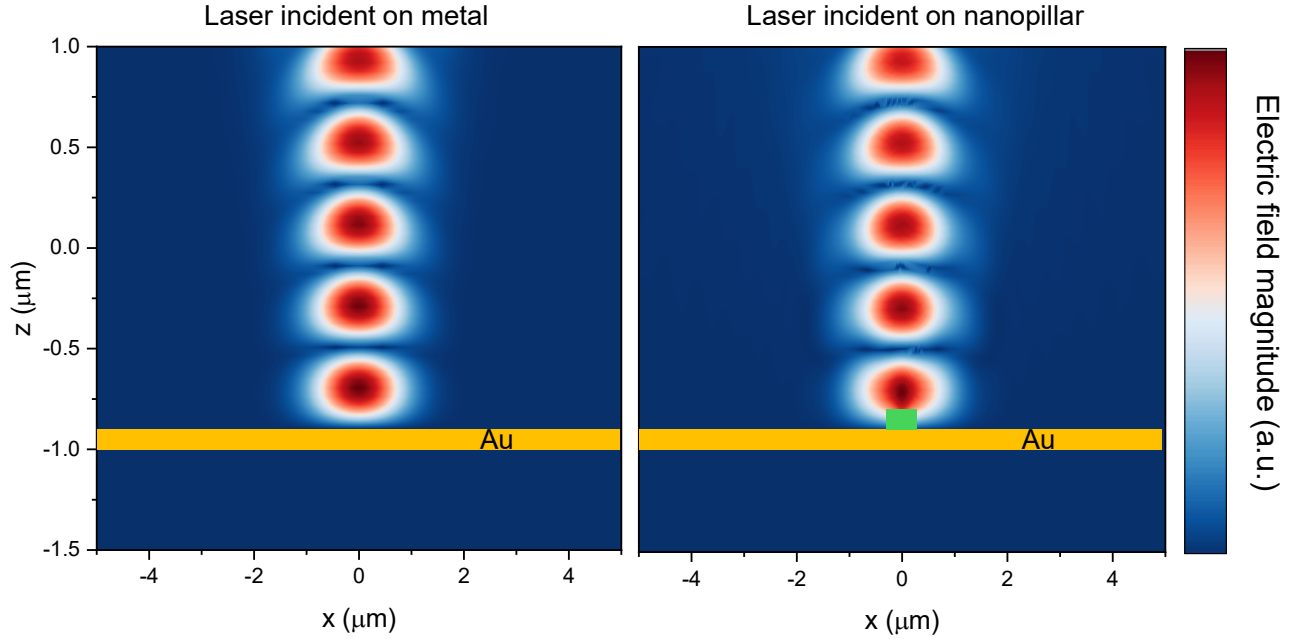

Supporting Figure 2: **Gaussian laser beam incident on a gold substrate and nanopillar:** Left: Presence of a reflective coating on the substrate causes nodes and antinodes to form in the electric field strength above the surface of the gold. Right: The top of the nanopillar is near the node of the Gaussian laser beam incident on the substrate.

Enhancement of SHG intensity on the nanopillar compared to the flat portion on gold can be attributed to two mechanisms. First is the formation of an antinode of the electric field strength near the gold surface due to the reflection of the laser beam and subsequent phase flip. This is evident in the FDTD simulation shown in Supporting Figure 2 (left). This causes the electric field at the monolayer location to be of minimum intensity and thus reduces the SHG intensity. On the other hand, the node of the electric field lies closer to the top of the nanopillar, giving rise to increased SHG signal from this region [Supporting Figure 2 (right)]. Second, the presence of strain on the monolayer at the nanopillar can enhance the SHG intensity, as shown in the literature [1–3].

### Supporting Information 3 Far-field SHG radiation pattern from different regions of the sample

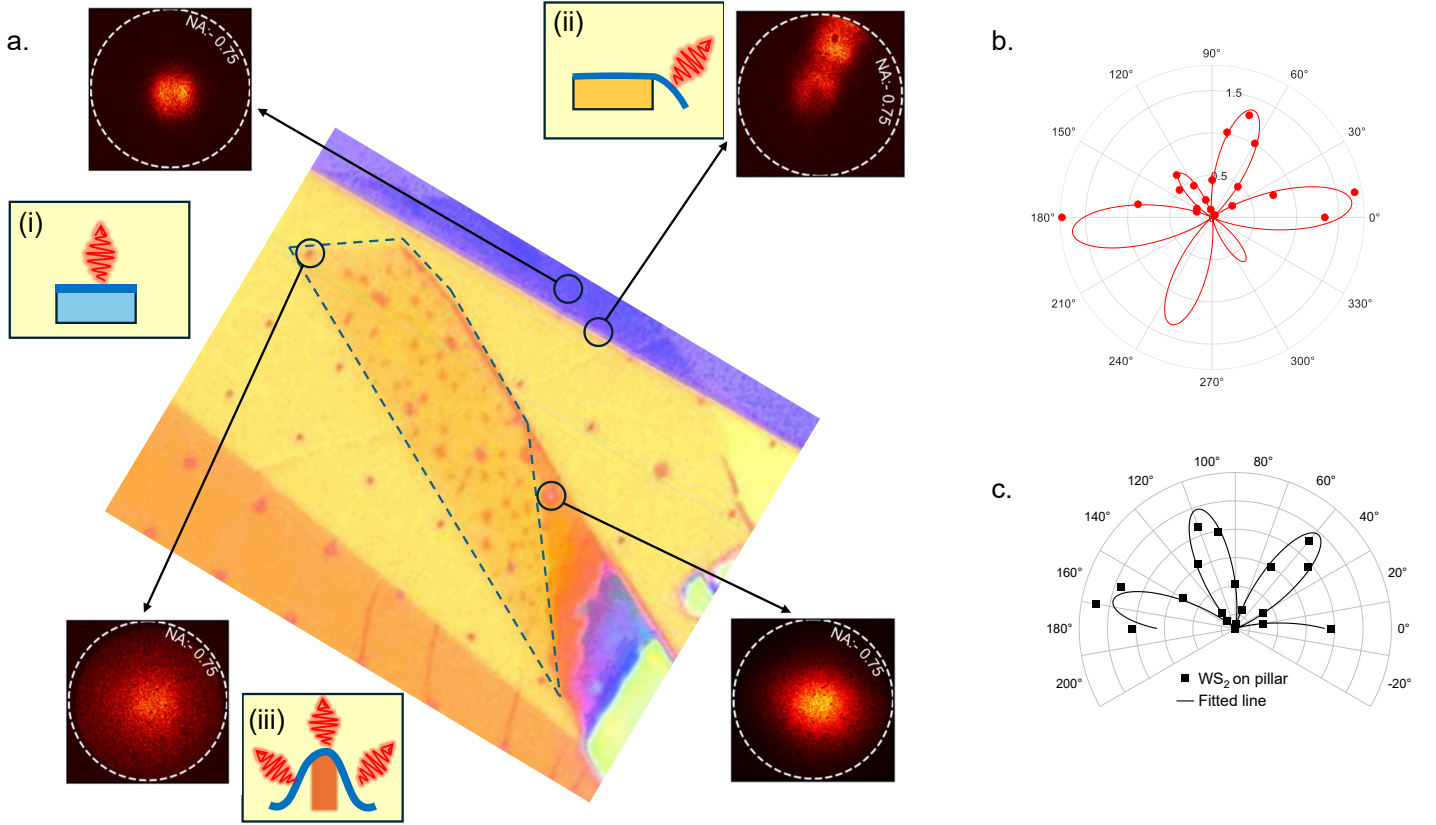

Supporting Figure 3: **Far-field SHG intensity pattern and SHG polar plot from different regions of the sample:** (a) Far-field SHG intensity pattern from monolayer on SiO<sub>2</sub>, monolayer on the gold-strip edge, and heterobilayer on two nanopillars are shown. (b) Polarization-resolved SHG signal plot for the region where the monolayer bends over the gold line edge. (c) Polarization-resolved SHG signal plot for WS<sub>2</sub> on the nanopillar.

Supporting Figure 3a shows the far-field SHG signal pattern from different regions of the sample. We take the radiation pattern of the monolayer on flat SiO<sub>2</sub> [schematically shown in Supporting Figure 3a inset (i)] as a reference to compare with other regions. Note that for the region where the monolayer resides on the edge of the gold line, the monolayer falls over on one side of the edge, resulting in anisotropic topography. This should result in a change in the direction of radiation from the monolayer towards higher angles in one particular direction normal to the edge of the gold line [Supporting Figure 3a inset (ii)]. This is evident in the

far-field radiation pattern, which shows radiation in one direction predominantly, and matches the direction of the slant portion of the monolayer falling from the gold line edge. Compared to this, the topography of the monolayers on and around the nanopillar is expected to be isotropic in geometry. In such a case, we do not expect a preferred direction of radiation, but SHG signal over higher angles is expected isotropically [Supporting Figure 3a inset (iii)]. Accordingly, the far-field radiation pattern from the nanopillars maintains an isotropic circular shape but with increased angular size resulting from the slant portions of the monolayers around the nanopillar. We see a distortion in the polarization resolved SHG intensity polar plot from the gold line edge due to unidirectional strain (Supporting Figure 3b). In contrast to this, polarization resolved SHG plot from pillar location, as shown in Supporting Figure 3c, does not show any such distortion and is similar to the case of monolayer on flat surface (Supporting Information 1). This suggests that the monolayers on the nanopillar experience isotropic strain with no preferred direction. The maintained isotropy of both the far-field radiation pattern and the polarization resolved SHG plot confirms that the isotropic strain from the nanopillar maintains the isotropy of the sample and thus of moiré pockets on the nanopillar as well.

## Supporting Information 4 FDTD simulation for excitons on pillar versus on gold substrate

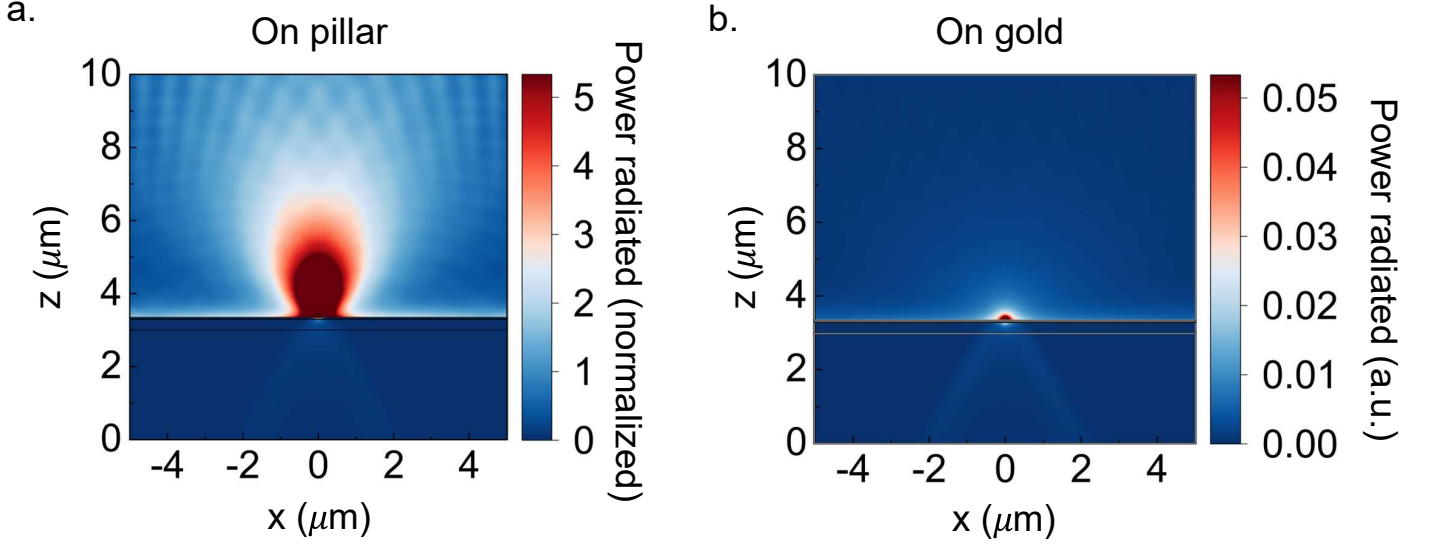

Supporting Figure 4: **FDTD simulation for excitons on pillar versus on gold substrate:** (a) Radiation pattern from excitons situated in the monolayer placed on the nanopillar. (b) Radiation pattern from excitons situated in the monolayer placed on the gold-coated substrate. Both the color plots are scaled such that they correspond to the same excitation laser power.

As discussed in Supporting Information 2, the incident laser beam on the gold surface results in an antinode near the surface. Accordingly, the excitation power seen by the monolayer and consequently its absorption is a lot less when placed directly on the gold-coated substrate compared to on top of the nanopillar. In Supporting Figure 4, results from FDTD simulation for excitons on a nanopillar versus on a gold surface are shown, under the same incident power. The effect of the lack of absorption in a monolayer directly placed on gold is already included in the results. Note that the scale bar for the plot of the exciton radiating from the gold surface is 100 times lower than the scale bar for the plot of the exciton on the nanopillar. Therefore, we conclude that the radiative emission from the monolayer touching the gold surface is quenched significantly compared to the monolayer placed on the nanopillar. Note that this result is

without considering the non-radiative exciton transfer to gold, which will make the quenching process even more prominent in the experiment.

## Supporting Information 5 Comparison of moiré emission from nanopillar versus from flat gold region

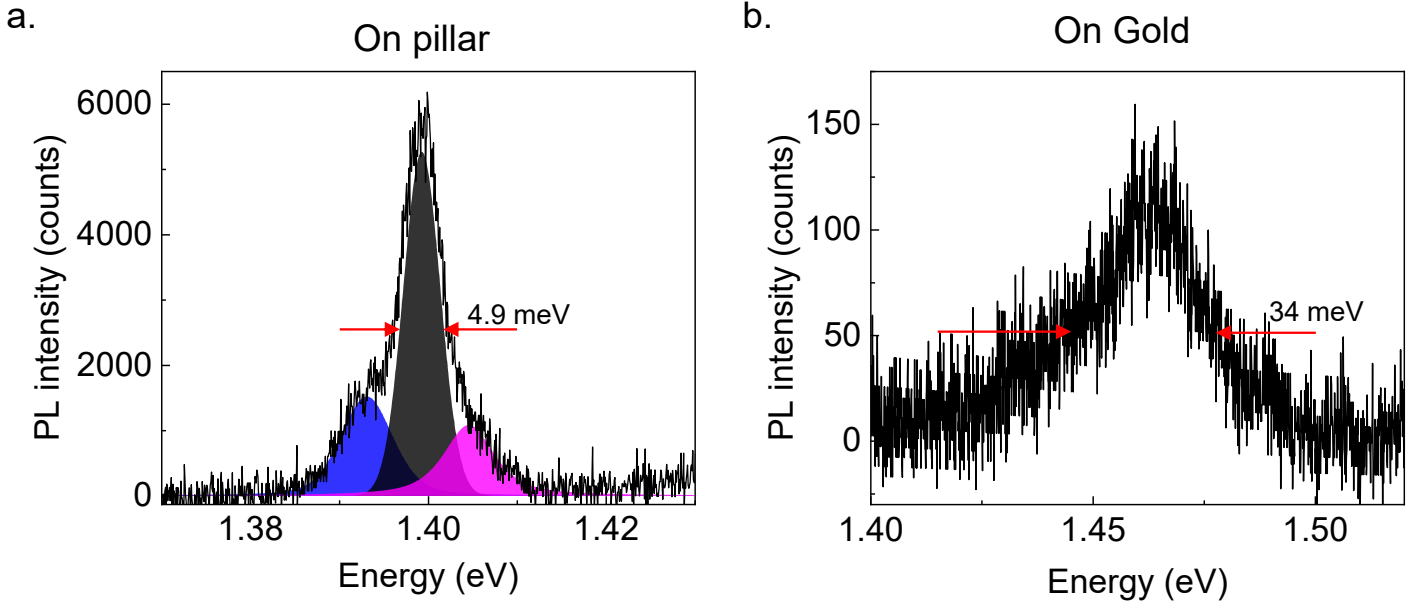

Supporting Figure 5: **Comparison of moiré emission from nanopillar versus from flat gold region:** (a) PL from heterobilayer on the nanopillar from another sample is shown with moiré exciton linewidth of  $\sim 4.9$  meV. (b) PL from heterobilayer on flat gold surface from the same sample as (a).

Supporting Figure 5a shows sharp emission (linewidth of 4.9 meV) from the heterobilayer on the nanopillar of another sample. We note that this is red-shifted (and significantly narrower) compared to the emission from the heterobilayer on the flat gold region of the same sample, as shown in Supporting Figure 5b. This redshift likely comes from the strain-induced band gap-lowering effect, which is also shown in intralayer excitons at room temperature in Figure 3 of the main text.



## Supporting Information 6 Superlinearity of exciton from another sample

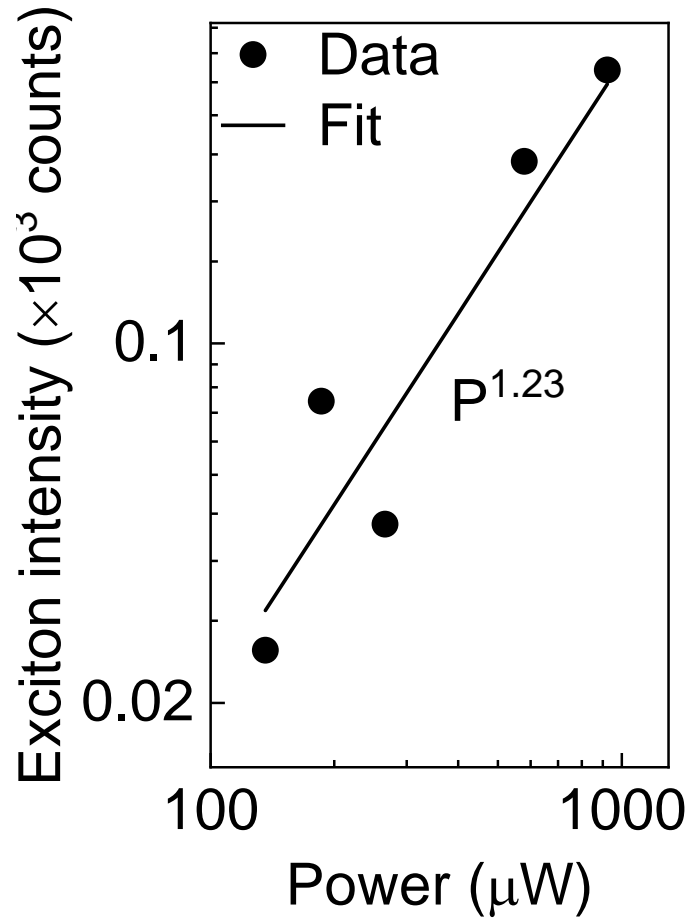

Supporting Figure 6: **Superlinearity of exciton from another sample:** Black circles show the PL intensity of the exciton peak after fitting, and the line is a power law fit to the data. Fit gives a value of  $\gamma=1.23$ .

Supporting Information 7 Power law coefficients of peaks  $X_1$   
and  $XX_{01}$

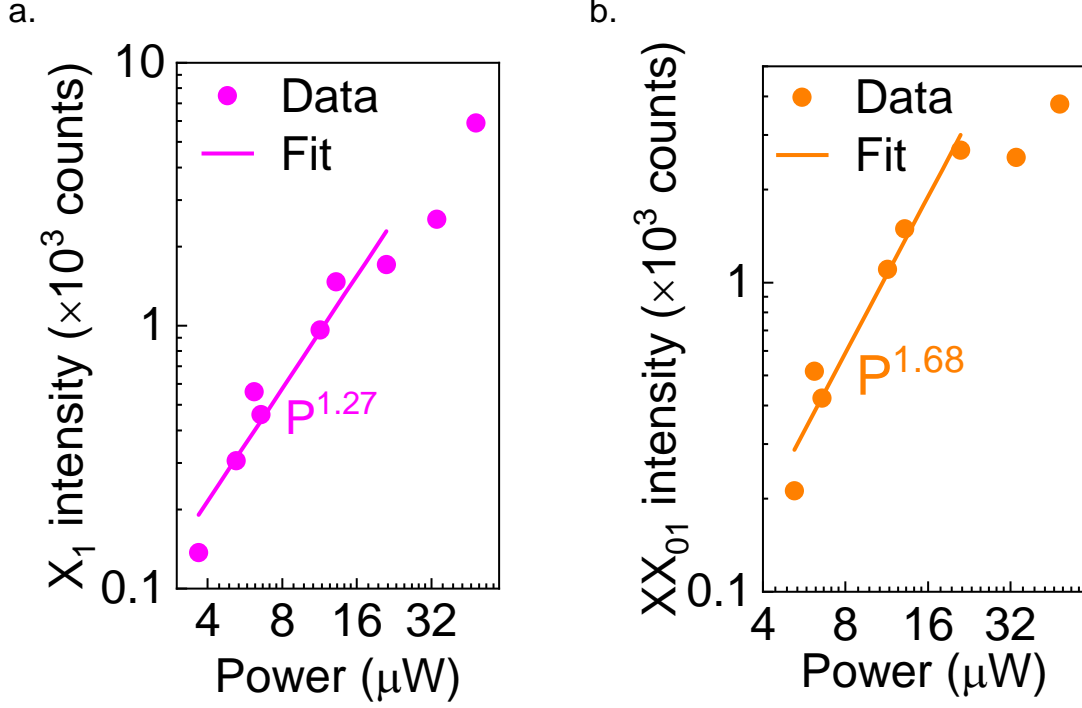

Supporting Figure 7: **Power law coefficients of peaks  $X_1$  and  $XX_{01}$ :** (a) PL intensity versus power plot for the peak  $X_1$ . Fit to the data gives  $\gamma=1.27$ . (b) PL intensity versus power plot of the peak  $XX_{01}$ . Fit to the data gives  $\gamma=1.68$ .

# Supporting Information 8 Data from another sample showing stabilized moiré trion and biexciton

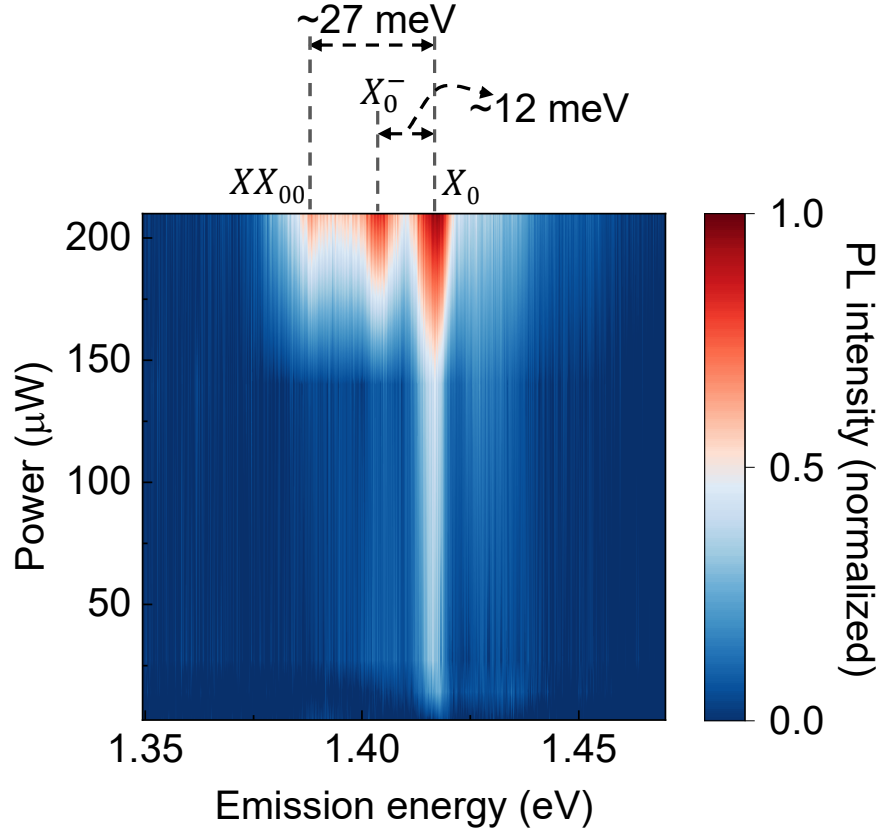

Supporting Figure 8: **Sample showing higher biexciton binding energy and lower dipolar repulsion:** Power dependent PL color plot of a sample showing biexciton (binding energy of  $\sim 27 \text{ meV}$ ), trion (binding energy of  $\sim 12 \text{ meV}$ ), and exciton.

## Supporting Information 9 Rate equations and lifetime measurements of the exciton ( $X_0$ ) and biexciton ( $XX_{00}$ )

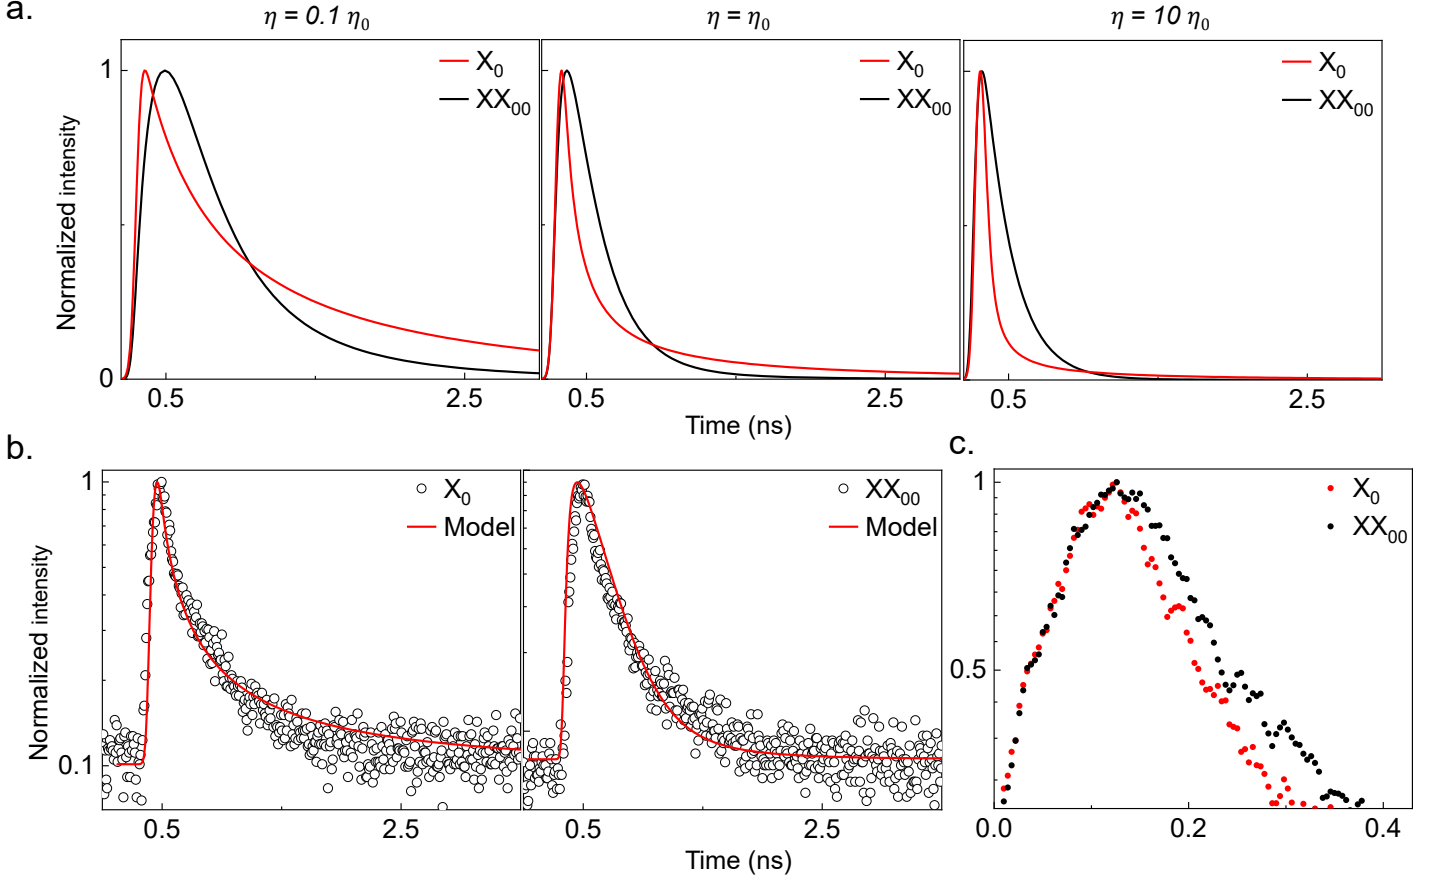

Supporting Figure 9: **Solutions of rate equations and lifetime measurement of the exciton ( $X_0$ ) and biexciton ( $XX_{00}$ ):** (a) Solutions of the rate equation for different values of exciton to biexciton conversion rates ( $\eta$ ). (b) Measured TRPL data for the exciton and biexciton (black circles) and fitting from the rate equations (red trace). (c) Zoomed in view of the overlaid exciton and biexciton TRPL data.

We model the exciton population  $[N_x(t)]$  and biexciton population  $[N_{xx}(t)]$  through coupled

rate equations as follows:

$$\frac{\partial N_x(t)}{\partial t} = g(t) - \frac{N_x(t)}{\tau_x} - 2\eta N_x^2(t) + \frac{N_{xx}(t)}{\tau_{xx}^r} \quad (1)$$

$$\frac{\partial N_{xx}(t)}{\partial t} = \eta N_x^2(t) - \frac{N_{xx}(t)}{\tau_{xx}} \quad (2)$$

where  $\tau_x$  is the exciton lifetime,  $\tau_{xx}$  is the biexciton lifetime with  $\tau_{xx}^r$  being its radiative component, and  $\eta$  quantifies the rate of exciton to biexciton conversion. The rate of generation of excitons by a Gaussian laser pulse is given by  $g(t) \propto e^{-\frac{1}{2}(\frac{t-\mu}{\sigma})^2}$  where  $\sigma$  is the width of the pulse and is related to its FWHM (59 ps) as  $\text{FWHM} = 2.355\sigma$ .

Supporting Figure 9a shows the solutions of these equations for different values of  $\eta$  with other parameters constant. We note that as the rate of exciton to biexciton conversion decreases, the decay curve of the biexciton becomes broader since the biexciton formation is delayed. Another interesting observation is the non-monexponential shape of the decay curve. Due to the presence of nonlinear terms in the coupled rate equations, we do not expect the experimental data to show a mono-exponential decay.

This is confirmed by the experimental data for exciton and biexciton TRPL data in Supporting Figure 9b. Both the exciton and the biexciton show a non-monexponential decay rate, which supports the coupling of their rate equations through nonlinear terms. At steady state ( $\frac{\partial N_{xx}(t)}{\partial t} = 0$ ),  $N_{xx} = \eta\tau_{xx}N_x^2$ . Therefore, the value of  $\eta\tau_{xx}$  can be estimated from PL measurements performed with a CW laser as  $\eta\tau_{xx} \sim 10^{-3}$ . Taking this as a starting point, we were able to simultaneously fit both the exciton and biexciton to the experimental data with the solutions of the rate equations with the fitting constants  $\tau_x = 4$  ns,  $\tau_{xx} = 0.34$  ns (with radiative part  $\tau_{xx}^r = 10$  ns), and  $\eta = 5.71 \times 10^6$  s<sup>-1</sup>. This shows that due to the nonlinear nature of the coupled differential equations, the decay rates measured in the TRPL experiment ( $\sim 50$ -100 ps here) can be much faster than the radiative lifetimes of the exciton and the biexciton. From the values of fitting parameters,  $\tau_{xx} < \tau_x$ , but both the experimental data and solutions to the rate equations show that the actual decay for the excitons is faster because of their conversion to biexcitons. Supporting Figure 9c shows a zoomed-in view of the exciton and biexciton TRPL data depicting the delayed biexciton emission, confirming that the exciton population is being converted to the biexciton population.

# Supporting Information 10 Biexciton stabilization with varying parameters

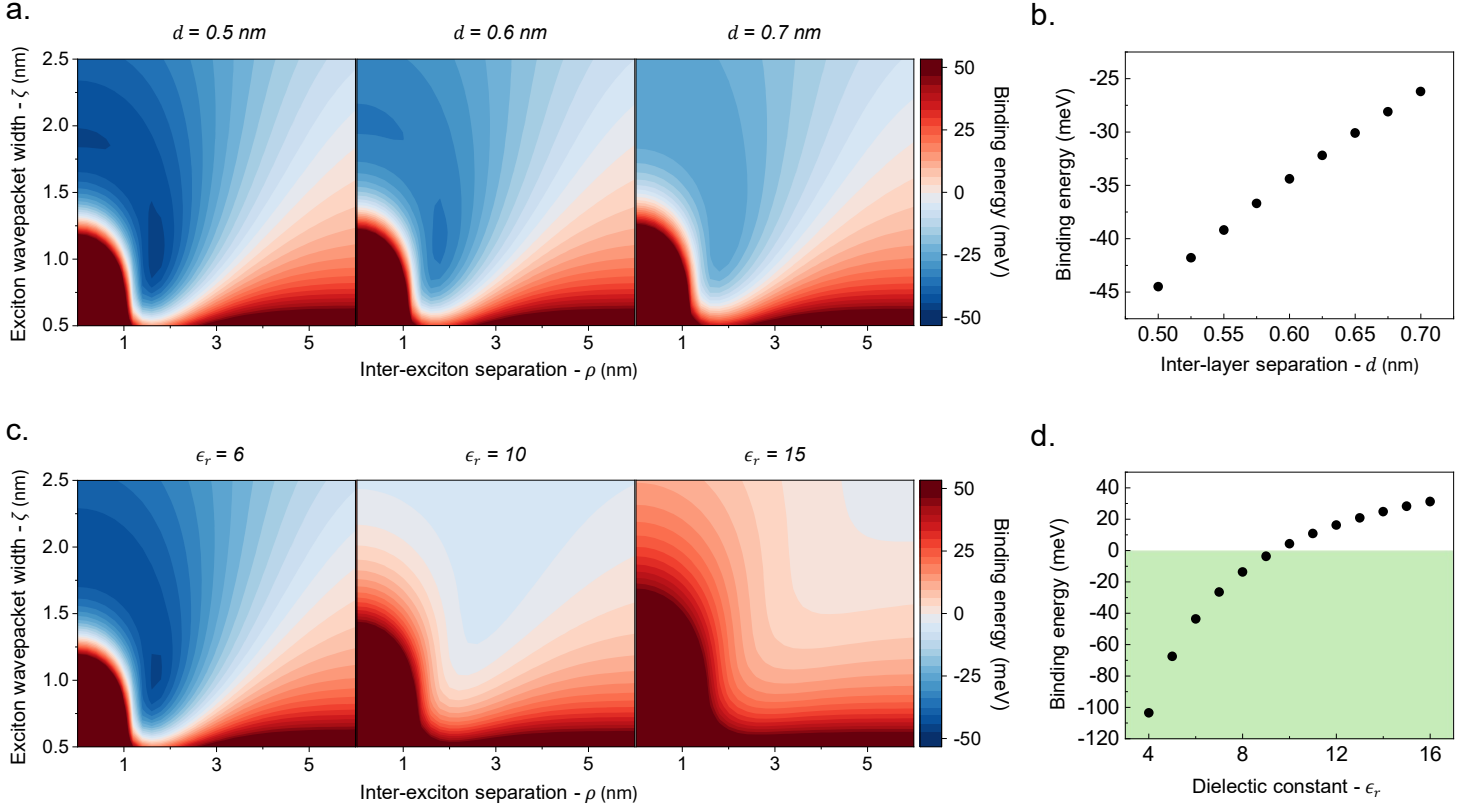

Supporting Figure 10: **Biexciton binding energy calculation with varying constants:** (a) Biexciton binding energy as a function of exciton wavepacket width ( $\zeta$ ) and inter-exciton separation ( $\rho$ ) with different values of interlayer separation ( $d$ ) for a given effective dielectric constant ( $\epsilon_r = 6.5$ ). (b) Variation of binding energy with interlayer separation for  $\zeta = 1.11$  nm and  $\rho = 1.8$  nm. (c) Biexciton binding energy as a function of exciton wavepacket width ( $\zeta$ ) and inter-exciton separation ( $\rho$ ) with different values of dielectric constant ( $\epsilon_r$ ) keeping a fixed inter-layer separation ( $d = 0.6$  nm). (d) Variation of binding energy with dielectric constant for  $\zeta = 1.11$  nm and  $\rho = 1.8$  nm. The green shaded portion shows the region of stability of the biexciton.

## Supporting Information 11 Biexciton binding energy as a function of exciton width in a moiré well

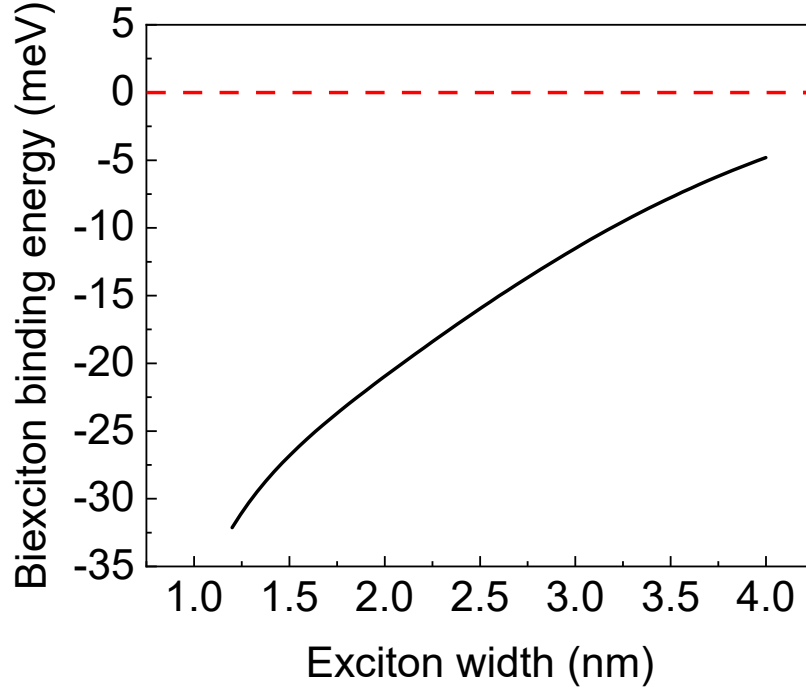

Supporting Figure 11: **Biexciton binding energy as a function of exciton width in a moiré well:** Binding energy of the biexciton is shown with varying exciton wavepacket width (and thus moiré well size or the twist angle.) The red dashed line denotes the limit after which the biexciton becomes unstable. A relatively smaller well size (and hence, a relatively larger twist angle) stabilizes the biexciton in a more efficient way.

For a given set of materials (such as  $\text{WS}_2$  and  $\text{WSe}_2$  here), the moiré twist angle determines the moiré well size, potential depth, and the moiré period. A wider moiré pocket would mean a wider center of mass wavefunction of the single exciton in the pocket, which would lead to a lower energy of the exciton. Since binding energy is the difference between the energy of the biexciton and the energy of two non-interacting excitons, the magnitude of the binding energy decreases when the individual exciton energy decreases. Thus, a wider moiré pocket leads to

biexcitons with lower binding energy. The same is confirmed by varying the individual size of the exciton wavepacket in our model, as shown in Supporting Figure 11. Therefore, a relatively smaller well size (and hence, a relatively larger twist angle) stabilizes the biexciton in a more efficient way.



## References

- [1] Zhizi Guan et al. “Strain-Induced Giant Second-Order Susceptibility in Monolayer WSe<sub>2</sub>”. *Physical Review B* 111.24 (2025), p. 245423.
- [2] Sudeep Puri et al. “Substrate Interference and Strain in the Second-Harmonic Generation from MoSe<sub>2</sub> Monolayers”. *Nano Letters* 24.41 (2024), p. 13061.
- [3] Sehwan Chang et al. “Enhancement of Second-Harmonic Generation in a 64° Stacked WSe<sub>2</sub>/WS<sub>2</sub> Heterobilayer with Local Strain”. *Nanotechnology* 35.14 (2024), p. 145201.
